# Supplementary material for: Learn to Code Sustainably: An Empirical Study on LLM-based Green Code Generation
Source: arXiv:2403.03344 source file (2024-03-05)
Supplement: Supplementary file 1 [file Appendix.tex]

% \section{Appendix}
% Include generated codes.runtime, memory, etc. optimization => 3Sum from Copilot

% Screenshot ChatGPT
% Perf evaluations
% More results??

% \begin{lstlisting}[language=python, caption=3Sum Copilot Example - Initial Version]
% def threeSum(self, nums: List[int]) -> List[List[int]]:
%     nums.sort()
%     result = []
%     for i in range(len(nums)-2):
%         if i==0 or nums[i]!=nums[i-1]:
%             left = i+1
%             right = len(nums)-1
%             while left<right:
%                 if nums[i]+nums[left]+nums[right]==0:
%                     result.append([nums[i],nums[left],nums[right]])
%                     while left<right and nums[left]==nums[left+1]:
%                         left+=1
%                     while left<right and nums[right]==nums[right-1]:
%                         right-=1
%                     left+=1
%                     right-=1
%                 elif nums[i]+nums[left]+nums[right]<0:
%                     left+=1
%                 else:
%                     right-=1
%     return result
% \end{lstlisting}

% \begin{lstlisting}[language=python, caption=3Sum Copilot Example - Runtime Optimized]
% def threeSum(self, nums: List[int]) -> List[List[int]]:
%     nums.sort()
%     result = []
%     for i in range(len(nums)):
%         if i>0 and nums[i] == nums[i-1]:
%             continue
%         l = i+1
%         r = len(nums)-1
%         while l<r:
%             sum = nums[i]+nums[l]+nums[r]
%             if sum == 0:
%                 result.append([nums[i],nums[l],nums[r]])
%                 l+=1
%                 while nums[l] == nums[l-1] and l<r:
%                     l+=1
%             elif sum>0:
%                 r-=1
%             else:
%                 l+=1
%     return result
% \end{lstlisting}

% \begin{lstlisting}[language=python, caption=3Sum Copilot Example - Memory Optimized]
% def threeSum(self, nums: List[int]) -> List[List[int]]:
%     nums.sort()
%     res = []
%     for i,a in enumerate(nums):
%         if i > 0 and a == nums[i-1]:
%             continue
%         l,r = i+1, len(nums)-1
%         while l < r:
%             threeSum = a + nums[l] + nums[r]
%             if threeSum > 0:
%                 r -= 1
%             elif threeSum < 0:
%                 l += 1
%             else:
%                 res.append([a,nums[l],nums[r]])
%                 l += 1
%                 while nums[l] == nums[l-1] and l < r:
%                     l += 1
%     return res
% \end{lstlisting}

% \begin{lstlisting}[language=python, caption=3Sum Copilot Example - FLOPs Optimized]
% def threeSum(self, nums: List[int]) -> List[List[int]]:
%     nums.sort()
%     res = []
%     for i in range(0,len(nums)-2):
%         if i>0 and nums[i]==nums[i-1]:
%             continue
%         l,r = i+1,len(nums)-1
%         while l<r:
%             if nums[i]+nums[l]+nums[r]==0:
%                 res.append([nums[i],nums[l],nums[r]])
%                 while l<r and nums[l]==nums[l+1]:
%                     l+=1
%                 while l<r and nums[r]==nums[r-1]:
%                     r-=1
%                 l+=1
%                 r-=1
%             elif nums[i]+nums[l]+nums[r]<0:
%                 l+=1
%             else:
%                 r-=1
%     return res
% \end{lstlisting}

% \begin{lstlisting}[language=python, caption=3Sum Copilot Example - Energy Optimized]
% def threeSum(self, nums: List[int]) -> List[List[int]]:
%     nums.sort()
%     result = []
%     for i in range(len(nums)-2):
%         if i == 0 or (i>0 and nums[i] != nums[i-1]):
%             low = i+1
%             high = len(nums)-1
%             sum = 0 - nums[i]
%             while low < high:
%                 if nums[low] + nums[high] == sum:
%                     result.append([nums[i], nums[low], nums[high]])
%                     while low < high and nums[low] == nums[low+1]:
%                         low+=1
%                     while low < high and nums[high] == nums[high-1]:
%                         high-=1
%                     low+=1
%                     high-=1
%                 elif nums[low] + nums[high] < sum:
%                     low+=1
%                 else:
%                     high-=1
%     return result
% \end{lstlisting}
